# Supplementary material for: Benchmarking Distributed Stream Data Processing Systems
Source: arXiv:1802.08496 source file (2019-06-24)
Supplement: Supplementary file 2 [file appendix.tex]

%!TEX root = icde2018.tex

\section{Technical Observations}

\subsubsection{Event time vs System time latency}
\label{event_vs_system}
In this paper, we introduce a new definition of latency for SDPSs. It is required to conduct a  comparative analysis of event time, system time and system-provided latencies. System time latency is the time interval between a tuple's ingestion at a SUT and its emission from the sink operator of the SUT, with our  technique to evaluate latencies of stateful operators. System-provided latency is the metric we obtain from SDPS.  The latency metrics inside the systems provide end-to-end $avg$ latency. One issue is that we cannot see the tuple based latency when using system metrics. Another issue is that the calculation of system-provided metrics might not be the same among different systems. So, it would be biased to utilize this metric when benchmarking different systems. Another issue is that, especially for windowed operations system-provided latency metrics  gives higher latencies than actual  system latency. The reason is that, the system cannot track which input tuples contribute to a given output tuple, so it computes average of both input and output tuple timestamps.   Event time latency, on the other hand, is the end-to-end latency between a tuple's event time and its emission time from the sink operator of SUT, with our latency evaluation technique of stateful operators. Figure \ref{event_vs_system_latency} shows the comparison between the system time and event time latency. We conducted  experiments with Query 1 (8s, 4s) on a 2-node cluster. Even with a small cluster size,  we can see that there is a significant difference between event and  system time  latencies. To be more specific, Storm has 1034, 1201, 1407 ms, Spark has 1040, 2491, 3394 ms, and  Flink has 254, 351, 563 ms system time, system-provided, and event time latencies respectively. As a result, we can see that with Spark, input tuples spend most of the time in input queues. Because Storm Spout is pure pull based, the tuples spend significant amount of time inside the system, inside operator buffers. Flink has a difference between event and system time latency in orders of magnitude. The reason is that backpressure affects only event time latency.   We examined the similar behavior with large cluster sizes and with windowed join queries as well.

\begin{figure*}
	\centering
	
	\begin{subfigure}[b]{0.32\textwidth}
		\includegraphics[width=\textwidth]{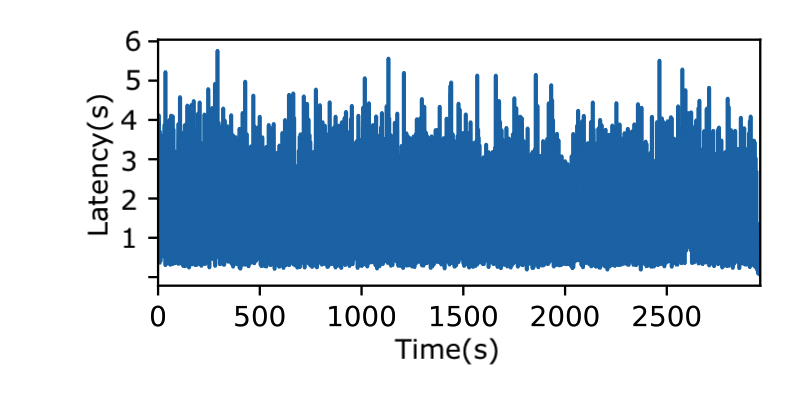}
		\includegraphics[width=\textwidth]{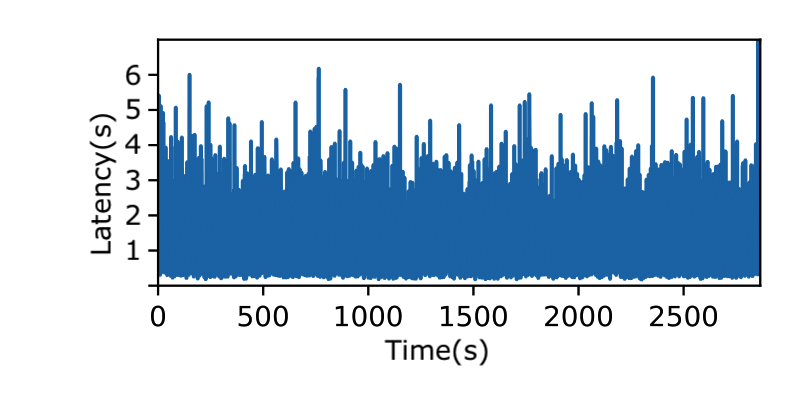}
		
		\caption{Event  vs system  time latency in Storm} 
	\end{subfigure}
	~ 
	\begin{subfigure}[b]{0.32\textwidth}
		\includegraphics[width=\textwidth]{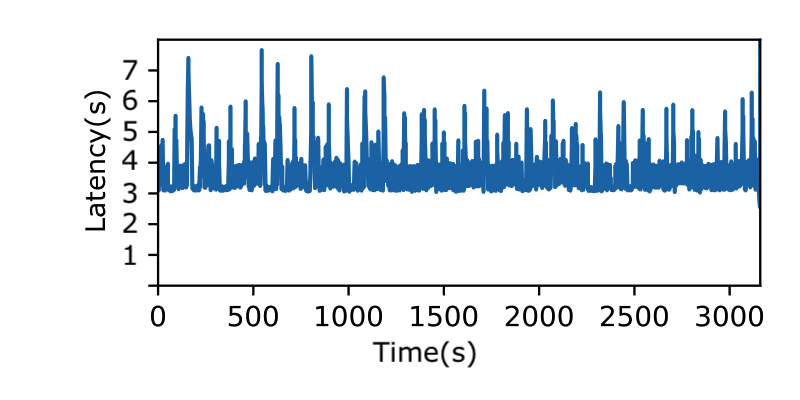}
		\includegraphics[width=\textwidth]{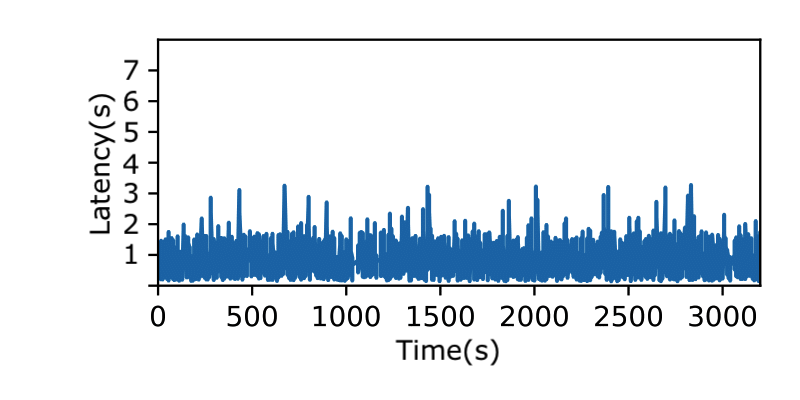}
		
		\caption{Event  vs system  time latency in Spark} 
	\end{subfigure}
	~ 
	\begin{subfigure}[b]{0.32\textwidth}
		\includegraphics[width=\textwidth]{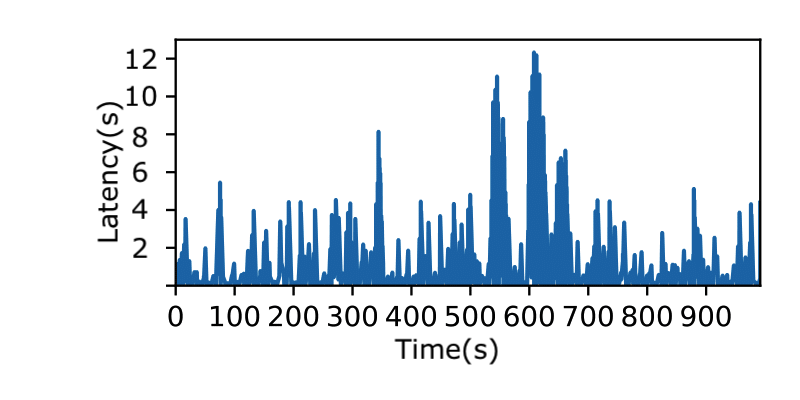}
		\includegraphics[width=\textwidth]{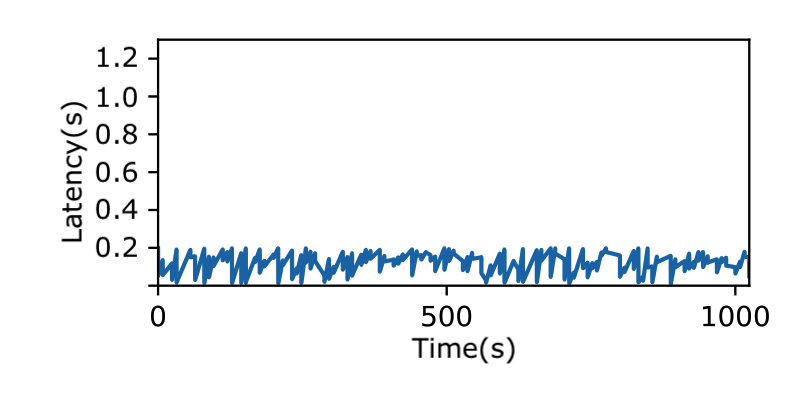}
		
		\caption{Event vs system time latency in Flink}
	\end{subfigure}
	
	\caption{Comparison between event and system time latency among systems}
	\label{event_vs_system_latency}
\end{figure*}

\subsubsection{Observing backpressure}
As discussed above, our driver can distinguish backpressure and unsustainable throughput. This is shown in Figures  \ref{fig_spark_join_2node_th_max_ts}, \ref{fig_spark_join_4node_th_max_ts}, \ref{fig_spark_join_8node_th_max_ts}, 	\ref{flink_join_2node_th_max_ts}, \ref{flink_join_4node_th_max_ts}, \ref{flink_join_8node_th_max_ts}, and \ref{flink_agg_2node_th_max_ts}. Moreover, our driver can also observe short-term spikes (Figures \ref{fig_storm_agg_8node_th_max_ts}, \ref{peaks_spark_join}) and  continuous fluctuations (Figure \ref{flink_join_2node_th_90_ts}). Furthermore, with the current values of $q^{a}$ and $q^{b}$,  we can observe a wide range of sustainable $avg$ latencies from 0.2 to 6.2 seconds and from 0.003 seconds $min$ latency to 19.9 seconds $max$ latency.

\subsubsection{Fault tolerance}
Measuring the SDPSs' fault tolerance is  well explored problem \cite{lopez2016performance}. Because measuring throughput and latency is orthogonal to performing fault tolerance measurements, we  refer to the benchmark results to previous results. In short, Spark is more robust to node failures than the other systems.

\subsubsection{Data pulling from the data source}
\label{pull_ds}
While analyzing the systems' performance it is essential to inspect their data pull graphs from data sources. We retrieved this metric from the driver. Figure \ref{pull_graph} shows the corresponding behavior of systems under test with MST with Query 1 (8s, 4s). However we examined the similar behavior in other window settings and with Query 2 as long as the workload is maximum sustainable.  As we can see, Spark and Storm have more fluctuating data pull rates than Flink. Despite having high data pull rate, Flink have less fluctuations. When we lowered the workload both Flink and Spark got to monotonic data pull rate; however, Storm still exhibited significant fluctuations. 
The reason is that Storm treats the main part of incremental computations as blackbox and performs frequent buffer fill and purge. So,  the system cannot adjust the stable buffer fill/purge rate for all receivers.  The main reason for fluctuation for Spark is having several jobs at the same batch interval. Spark has $action()$ method on each RDD; as a result, the number of jobs at any time will be equal to the number of $action()$ method calls. Each job retrieves the data into its input buffers and fires. Until a job is finished, its input rate is limited. It is the DagScheduler's job to coordinate and schedule all running jobs. As a result, we can see non-monotonic data pull graphs for Spark. Flink, on the other hand, benefits from its internally incremental computation mechanism (like Spark), tuple at a time semantics and efficient backpressure mechanism.

\begin{figure*}
	\centering
	
	\begin{subfigure}[b]{0.32\textwidth}
		\includegraphics[width=\textwidth]{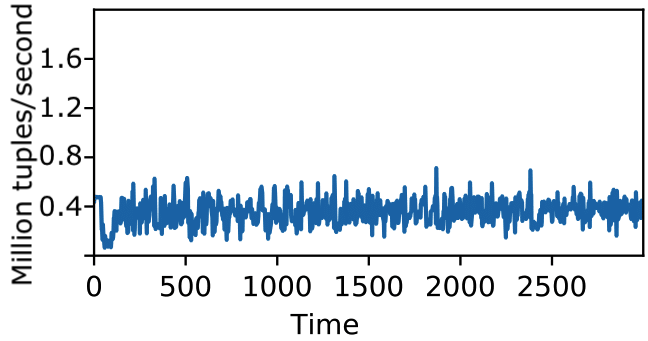}

		\caption{Storm} 
	\end{subfigure}
	~ 
	\begin{subfigure}[b]{0.32\textwidth}
		\includegraphics[width=\textwidth]{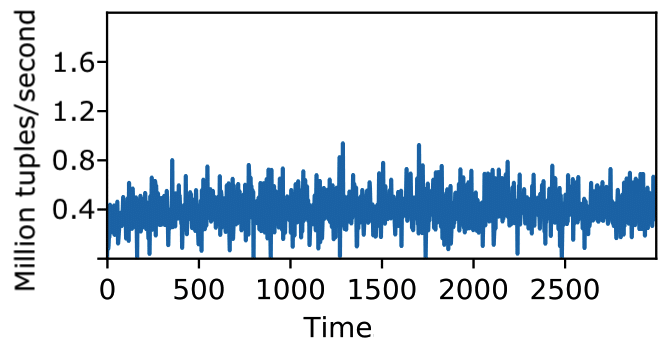}

		\caption{Spark} 
	\end{subfigure}
	~ 
	\begin{subfigure}[b]{0.32\textwidth}
		\includegraphics[width=\textwidth]{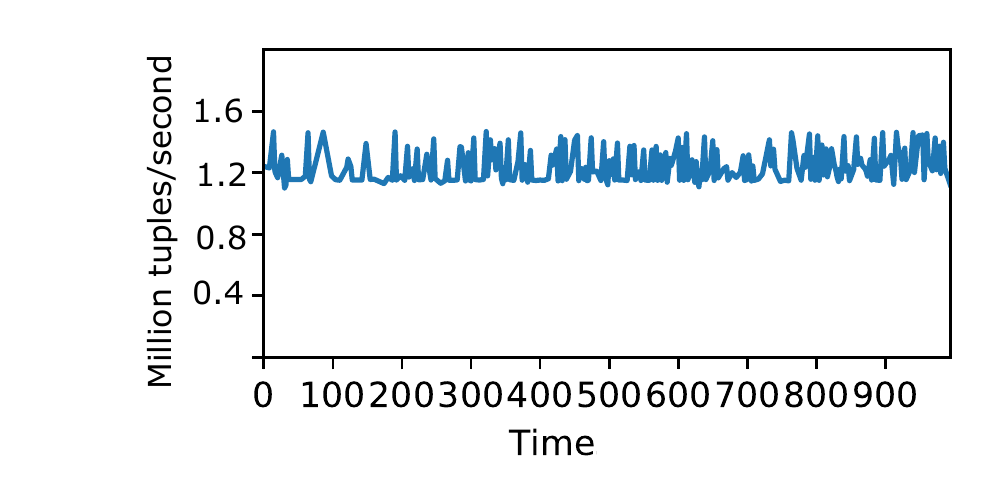}

		\caption{ Flink} 
	\end{subfigure}
	
	\caption{Data pull graphs of systems under test}
	\label{pull_graph}
\end{figure*}

\begin{figure*}
	\centering
	
	\begin{subfigure}[b]{0.32\textwidth}
		\includegraphics[width=\textwidth]{eps/storm_load_one}
		\includegraphics[width=\textwidth]{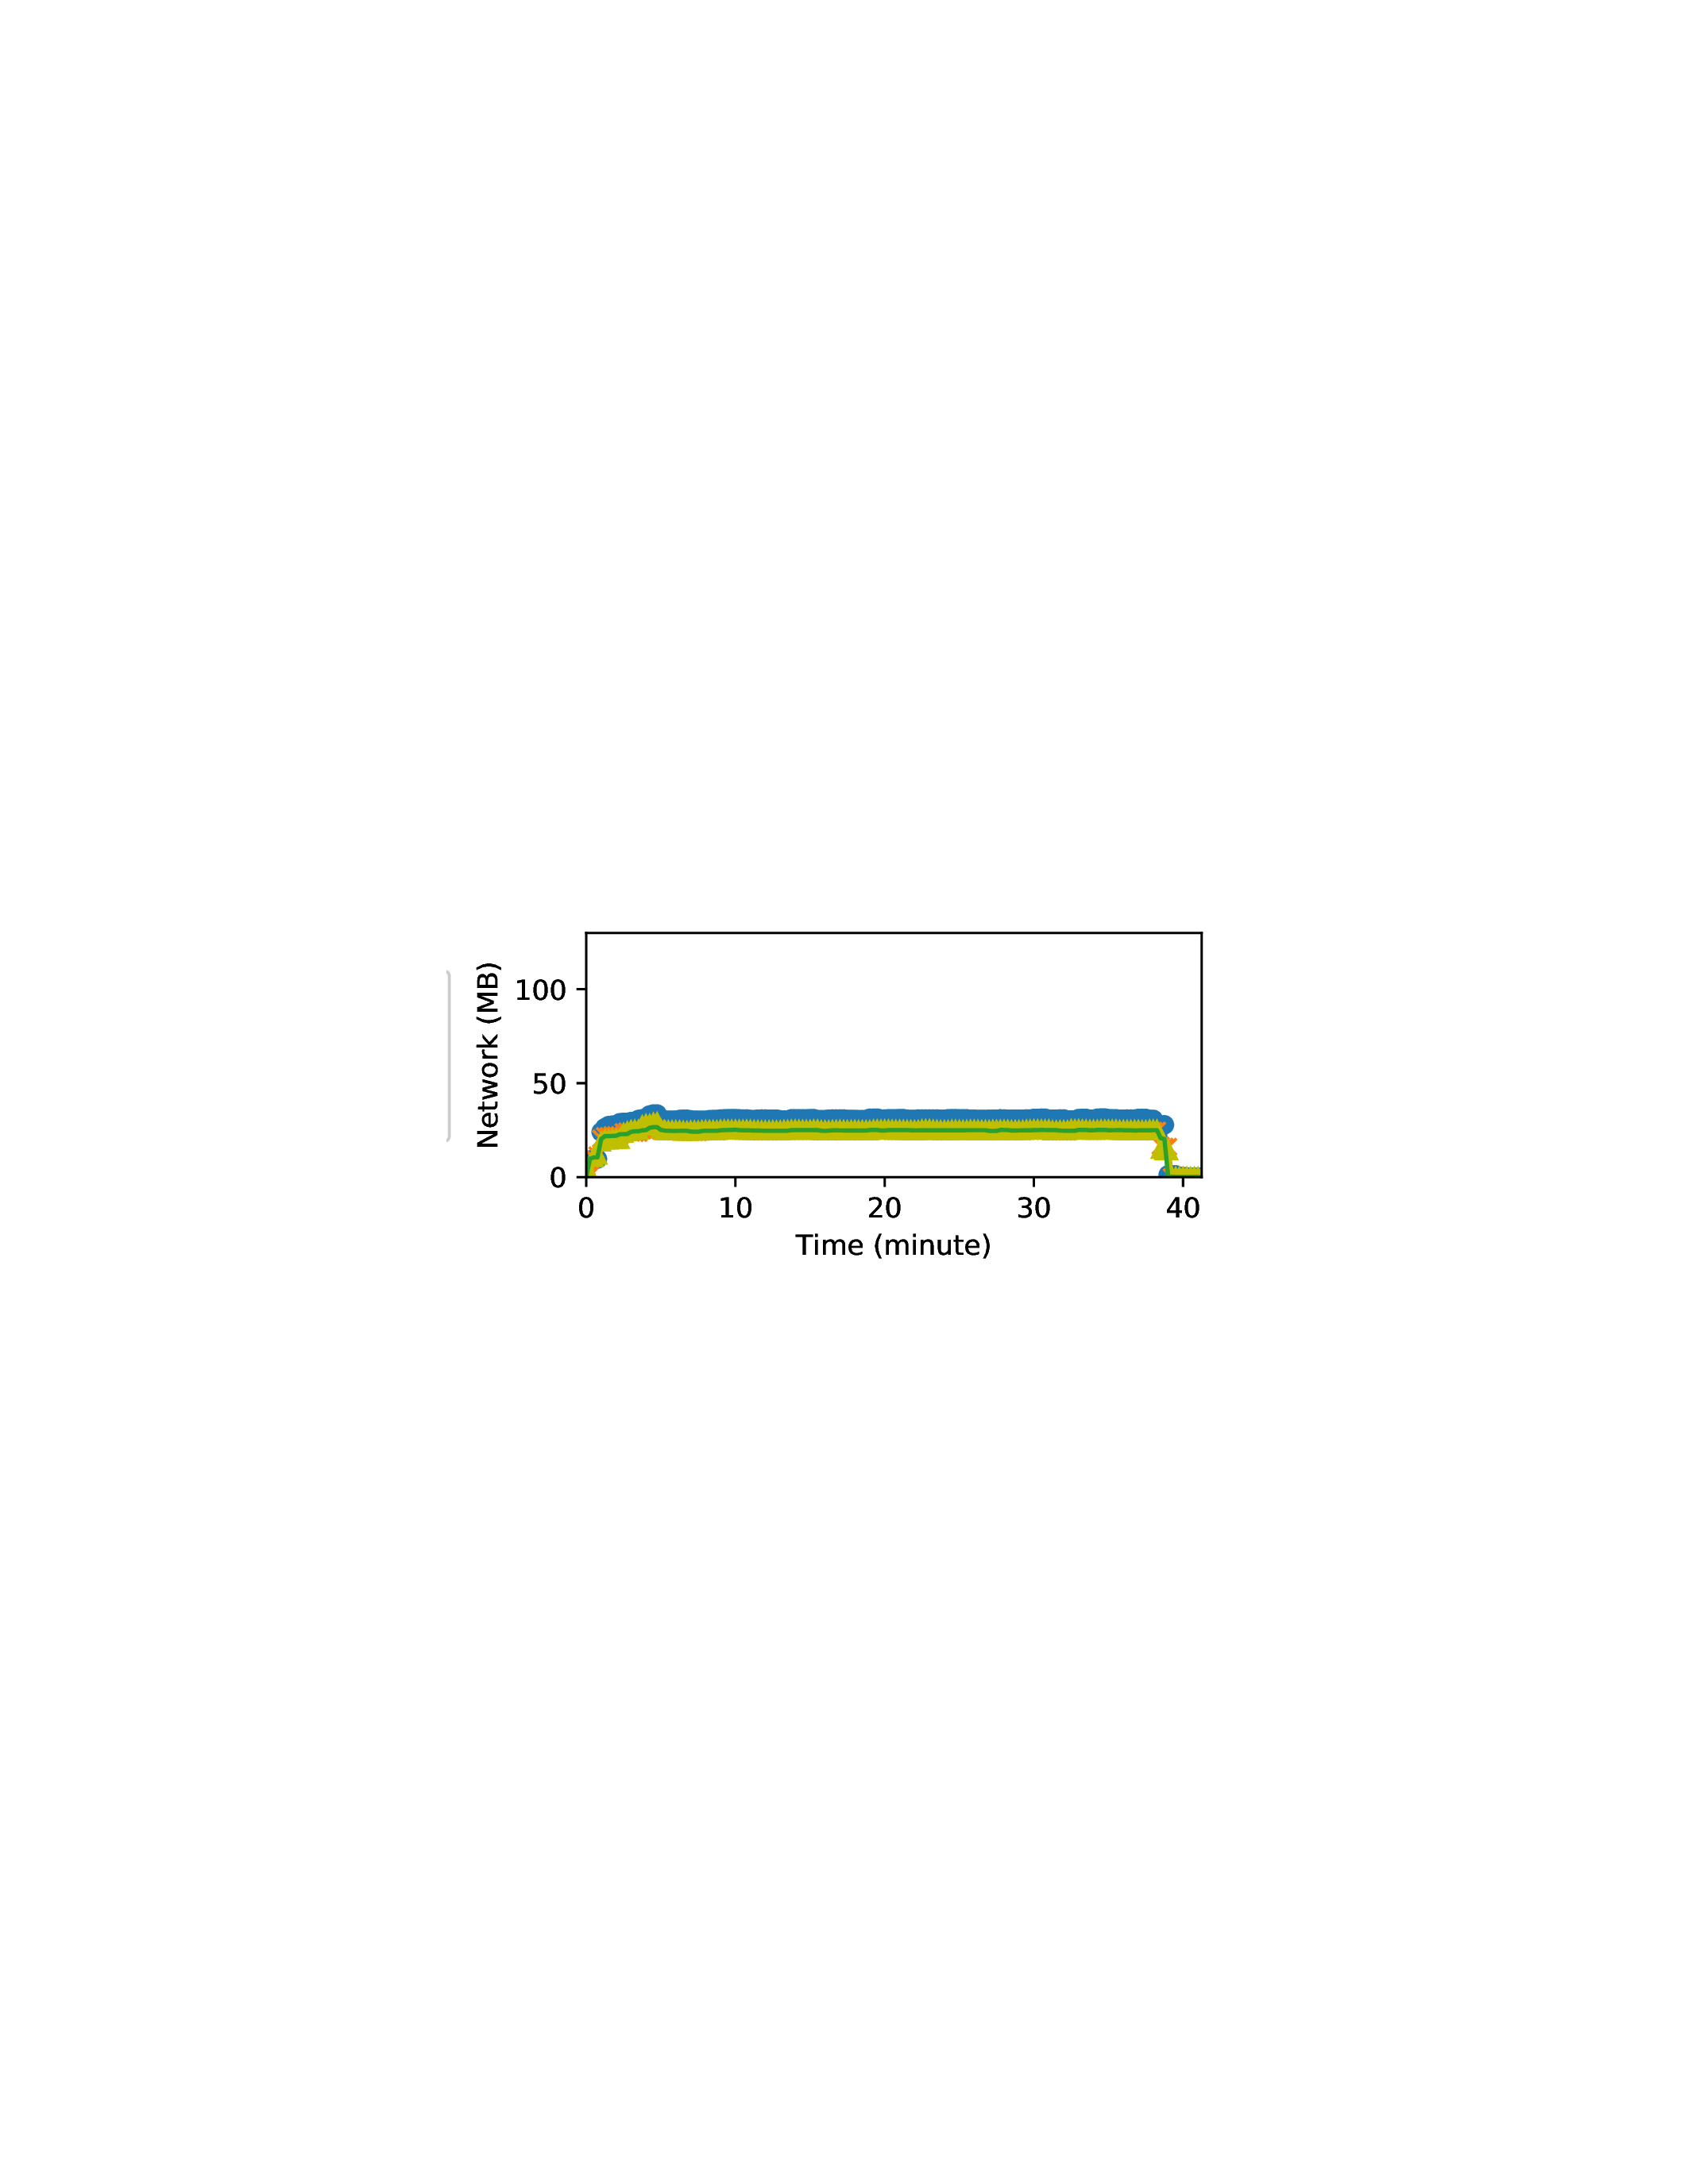}
		
		\caption{CPU and network usage of Storm }
	\end{subfigure}
	~ 
	\begin{subfigure}[b]{0.32\textwidth}
		\includegraphics[width=\textwidth]{eps/spark_load_one}
		\includegraphics[width=\textwidth]{eps/spark_bytes_in}
		
		\caption{CPU and network usage of Spark }
	\end{subfigure}
	~ 
	\begin{subfigure}[b]{0.32\textwidth}
		\includegraphics[width=\textwidth]{eps/flink_load_one}
		\includegraphics[width=\textwidth]{eps/flink_bytes_in}
		
		\caption{CPU and network usage of Flink }
	\end{subfigure}
	
	\caption{CPU and Network usage of systems in a 4-node cluster. Colors indicate nodes in a cluster}
	\label{fig_cpu_network_metrics}
\end{figure*}

\begin{figure*}
	\centering
	%\captionsetup[subfigure]{aboveskip=2pt,belowskip=-1pt}
	\begin{subfigure}[b]{0.45\textwidth}
		\includegraphics[width=\textwidth]{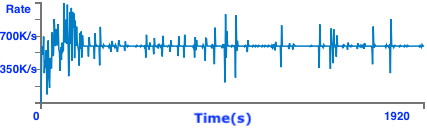}

		\caption{Scheduler delay} 
	\end{subfigure}
	~ 
	\begin{subfigure}[b]{0.45\textwidth}
		\includegraphics[width=\textwidth]{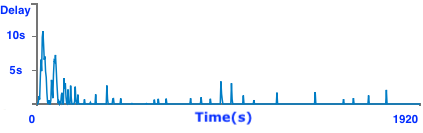}
		
		\caption{Input rate }
	\end{subfigure}

	\caption{Scheduler delay and input rate in Spark}
	\label{scheduler}
\end{figure*}

\subsubsection{Resource usage statistics} Figure \ref{fig_cpu_network_metrics} shows the resource usages of the SUTs. The upper figure shows the CPU load during the experiment. The CPU load is the number of kernel level threads  that are runnable and queued while waiting for CPU resources, averaged over one minute. The next figure shows the network usage of the SUTs.  Because the overall result is similar, we show the systems' resource utilization graphs  with windowed aggregation case in 4-node cluster.  Because Flink's performance is bounded by network, we can see that CPU utilization is minimal among others. Storm, on the other hand, uses approximately 50\% more CPU clock cycles than Spark. This results in having competitively higher throughout than Spark. 
We perform experiments with different parallelism settings, block, buffer, and batch sizes, as we explained in Tuning the Systems subsection.  For example, increasing block and buffer size improves the throughput but results in long-lasting jobs. Especially for join queries this can result in long job queues. Increasing parallelism improves the throughput  but this is highly dependent on the query. Throughout our experiments, we tune the systems to find the best combination of parameters for each system.
One reason behind Spark's efficient CPU usage is its automation, transparent resource usages, and many internal optimizations   \cite{sparkcodegen}. For example, Spark handles incremental state management, optimizations with code generation, and dynamic memory management efficiently and transparent to user.  
However, as we can see from Figure \ref{scheduler}, the scheduler overhead is one bottleneck for Spark's performance.  Initially, Spark ingests tuples more than it can sustain. Because of the scheduler delay, backpressure fires and limits the input rate. Whenever there is even a short spike in the input rate, we can observe a similar behavior in the scheduler delay.

\subsubsection{More scenarios}

We conducted experiments in a more complex scenarios with Query 3 from Listing 2. The main purpose is to inspect the engines' query optimization with non-trivial queries and their scaling capabilities.
One key finding is that  both Flink and Spark supports  operator chaining both In the logical and the physical query graph. For example, Flink  chains operators  (e.g., two subsequent map transformations) if the operation is possible. However, optimizations like join ordering, automatic intermediate result materialization (or caching), subgraph sharing, fission and etc. are not available in neither systems. 
Another key finding is that with a more complex query the performance of the systems stay  at the same proportion as the fundamental queries like windowed aggregation and windowed joins. We conducted experiments up to 20-node cluster configuration with Query 3 for all systems. We observed that with increasing number of computing nodes Spark outperforms Storm. For example, with 20 nodes Spark achieved a 1.5 higher throughput than Storm. Due to space restrictions, we do not provide detailed numbers here.

Moreover, we tested the systems with lower workloads than they can sustain. For all  systems the $avg$ latency increases with the smaller workloads given the same buffer size and batch interval. We had to tune the buffer size and batch interval for each workload to lower the latency. However, in real industrial scenario this is not the case. So, once the workload decreases the system should not be stopped and tuned for a particular workload but it should perform so automatically.

\begin{lstlisting}[
language=SQL,
showspaces=false,
basicstyle=\ttfamily,
numbers=left,
numberstyle=\tiny,
commentstyle=\color{gray}
label=list3,
caption={More complex query},
captionpos=b]
GET INPUT  l (window length) 
and s (window slide)
S_1 = UNION  {s_1, s_2, ..., s_m}
S_2 = UNION {s_m, s_m+1, ..., s_n}
S_3 = UNION  {s_1, s_2, ..., s_n}
Query_3 = 
1.UPDATE S_1, S2: enrich with a new field = 
cnt,  the country name of geo location
2.TEMP_RESULT=SELECT AVG(R.price)
FROM  
(SELECT MAX(S_2.price, S_3.price)
FROM S_2, S_3 on window(l, s), 
WHERE S_2.cnt = S3.cnt and S_2.ts = S3.ts)  
as R on window(l, s)  
GROUPBY R.geo
WHERE R.price > 100
3.Execute Query 1 with input streams=TEMP_RESULT
\end{lstlisting}

%!TEX root = icde2018.tex
\section{PRELIMINARIES AND BACKGROUND}
\label{pre}

In this section, we provide background information about the stream data processing engines and their features used in this paper. 
We analyze Apache Storm, Apache Spark, and Apache Flink as they are the most mature and accepted ones in both academia and industry.

\subsection{Apache Storm}

Apache Storm is a distributed stream processing framework, which was open sourced after being acquired by Twitter \cite{storm}. 

Storm operates on tuple streams and provides record-by-record stream processing. 
It supports an at-least-once processing  semantics and guarantees all tuples to be processed. 
In cases of failure, events are replayed. 
Storm also supports exactly-once processing semantics with its Trident abstraction \cite{trident}. 

Stream processing programs are represented by a computational topology, which consists of spouts and bolts. 
Spouts are source operators and bolts are processing and sink operators. 
A Storm topology forms a directed acyclic graph (DAG), where the edges are tuple streams and vertices are operators (bolts and spouts). 
When a spout or bolt emits a tuple, the bolts that are subscribed to this spout or bolt receive input.

Storm's lower level APIs provide only limited support for automatic memory and state management. 
Therefore, choosing the right data structure for state management and utilizing memory efficiently by making computations incrementally  is up to the user. 
Storm supports caching and batching the state transition. 
However, the efficiency of a particular operation degrades as the size of the state grows.

Storm has built-in support for windowing. 
Although the information of expired, newly arrived, and total tuples within a window is provided through APIs, the incremental state management is not transparent to the users. 
Trident, on the other hand,  has built-in support for partitioned windowed joins and aggregations. 
Storm supports sliding and tumbling windows on processing time and event time. 
For event-time windows, tuples need to have a dedicated timestamp field so that the engine can create periodic watermarks. 
Any worker process in Storm topology sends acknowledgments to the source executor for a processed tuple. 
In case of failure Storm sends the messages again. 
A downside of acknowledgments in Storm is that tuples can be only be acknowledged once they are completely flushed out of a window by the operator. 
This is especially problematic for long windows with small slide.

Backpressure is one of the key features of SDPSs. 
It refers to the situation where a system is receiving data at a higher rate than it can process. 
For example, this can occur during temporary load spikes. 
Storm supports backpressure although the feature is not mature yet \cite{WinNT}. 
This was confirmed throughout our experiments as well.

Storm uses an extra backpressure thread inside the system. 
Once the receiver queue of an operator is full, the backpressure thread is notified. 
This way Storm can notify all workers that the system is overloaded. 
Due to its high complexity, Storm's backpressure feature can stall the system and, therefore, it is not enabled by default in the current version.

\subsection{Apache Spark}
Apache Spark is an open source big data processing engine, originally developed at the University of California, Berkeley \cite{spark}. 
Unlike Storm and Flink, which support one record at a time, Spark Streaming inherits its architecture from batch processing, which supports processing records in micro-batches. 
Throughout this paper, we refer to Spark Streaming as simply Spark. 
The Resilient Distributed Dataset (RDD) is a fault-tolerant abstraction of Spark, which enables in-memory, parallel computation in  distributed cluster environments \cite{zaharia2012resilient}.

One of Spark's features is its support of lazy evaluation. 
This enables the engine to run more efficiently. 
Spark  supports stage-oriented scheduling. 
Initially, it computes a DAG  of stages for each submitted job. 
Then it keeps track of materialized  RDDs and outputs from each  stage, and finally finds a minimal schedule. 
Unlike Flink and Storm, which also work based on DAG execution graphs, Spark's computing unit in a graph (edge) is a data set rather than streaming records and each vertex in a graph is a stage rather than individual operators. 
RDDs are guaranteed to be processed in order in a single DStream (Discretized Stream), which  is a continuous sequence of RDDs. 
However, there is no guaranteed ordering within RDDs  since each RDD is processed in parallel.

Spark has improved its memory management significantly in the recent releases. 
The system shares the memory  between execution and storage. 
This unified memory management supports dynamic memory management between the two modules. 
Moreover, Spark supports dynamic memory management throughout the tasks and within operators of each task.

Spark has a built-in support for windowed calculations. 
It supports only windows defined by processing time. 
The window size must be a multiple of the batch interval, because a window keeps a particular number of batches until it is purged. 
Choosing the  batch interval can heavily affect the performance of window-based analytics. 
First, the latency and response time of windowed analytics is strongly relying on the batch interval. 
Second, supporting only processing time windowed analytics, can be a severe limitation for some use-cases.

Spark also supports backpressure. 
It handles backpressure by putting a bound to the block size. 
Depending on the duration and load of each mini-batch job, the effectiveness of backpressure signal handling from source to destination may vary. 

%todo[inline]{fast enough for what?=>fixed}

\subsection{Apache Flink}
Apache Flink started off as an open source big data processing system at TU Berlin, leveraging in major parts the codebase of the Stratosphere project [9].
At its core, Flink is a distributed dataflow engine. 
Like in Storm, a Flink runtime program is a DAG of operators connected with data streams. 
Flink's runtime engine supports unified processing of batch (bounded) and stream (unbounded) data, considering former as being the special case of the latter.

Flink provides its own memory management to avoid long running JVM's garbage collector stalls by serializing data into memory segments. 
The data exchange in distributed environments is achieved via buffers. 
A producer takes a buffer from the pool, fills it up with data, then the consumer receives the data and frees the buffer informing the memory manager. 
Flink provides a wide range of high level and user friendly APIs to manage  state. 
Incremental state update, managing the memory, or checkpointing with big states are performed automatically and transparently to user.

Flink has a strong feature set for building and evaluating windows on data streams. 
With a wide range of pre-defined windowing operators, it supports user-defined windows with custom logic. 
The engine provides processing-time, event-time, and ingestion-time semantics. 
When using processing time, like Spark, windows are defined with respect to the wall clock of the machine that is responsible for building and processing  a window. 
When using event time, on the other hand, the notion of time is determined by the timestamp attached to an event, which typically resembles its creation time. 
Like in Storm, the timestamps must be attached to each event record as a separate field. 
At ingestion time, the system processes records with event time semantics on these timestamps. 
Flink has support for out-of-order streams, which were motivated from Googles MillWheel and Dataflow papers \cite{akidau2013millwheel,akidau2015dataflow}. 
Flink also supports backpressure. 
It uses blocking queues. 
Once the congestion is detected this information is automatically transferred to upstream operators at negligible cost.
